# Supplementary material for: Modeling Approaches for Addressing Simple Unrelaxable Constraints with Unconstrained Optimization Methods
Source: arXiv:2205.09627 ancillary file (2022-11-10)
Supplement: Supplementary file 1 [file online_supplement.pdf]

# Online Supplement to: Modeling Approaches for Addressing Simple Unrelaxable Constraints with Unconstrained Optimization Methods


Jeffrey Larson[1], Misha Padidar[1,2], and Stefan M. Wild[1]

[1]Mathematics and Computer Science Division, Argonne National Laboratory
jmlarson@anl.gov; wild@anl.gov
[2]Center for Applied Mathematics, Cornell University
map454@cornell.edu


June 7, 2022

## 1 Data Profiles for Subsets of Problems

In this appendix we show data profiles for the subset of 22 CUTEst problems in Appendix C that have no constraints active at the solution and for the subset of 18 problems that have at least one constraint active at the solution.

Since PPM is smooth on the interior of $\boldsymbol{\Omega}$, optimizing it should be comparable in difficulty to that of the smooth problems PROB and eq. (1). We note that some solutions may be near boundaries, and so the optimization algorithm applied to PPM [1] may evaluate outside $\boldsymbol{\Omega}$ and incur the effects of the nonsmoothness near the boundary. The methods in the data profile are identical to those described in Section 5.

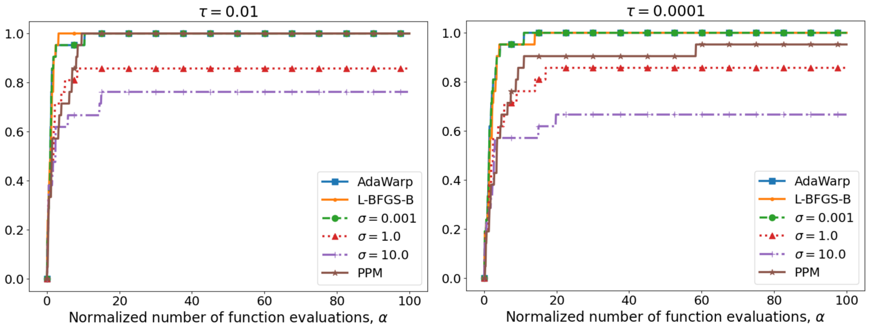


Figure 1: Data profile for a relative KKT tolerance of $\tau = 10^{-2}$ (left) and $\tau = 10^{-4}$ (right) for L-BFGS-B, Algorithm 1 under UPRULE and $\boldsymbol{\sigma}_0 = 10^{-3}$ and L-BFGS as a subproblem solver(labeled AdaWarp), BFGS optimizing $\widetilde{f}_{\boldsymbol{\sigma}}$ with a fixed $\boldsymbol{\sigma}$ (labeled $\boldsymbol{\sigma} = 0.001, 1.0, 10.0$), and the projection-based penalty formulation from [2] solved by [1](labeled PPM). These data profiles are for the set of 22 CUTEst problems with solutions on the interior of $\boldsymbol{\Omega}$.

The data profile for PPM is significantly improved on this set of problems, showing the benefit to the optimizer of solving over a largely smooth domain. Since the optimization algorithm applied to PPM is a variant of L-BFGS, we expect that it does perform slightly worse than L-BFGS-B because of the nonsmoothness it is forced to handle and a less direct method of handling the bound constraints. We also find that the optimization of $\widetilde{f}_{\boldsymbol{\sigma}}$ with $\boldsymbol{\sigma} = 0.001$ (labeled $\boldsymbol{\sigma} = 0.001$) significantly improves in performance for the data profile with relative KKT tolerance $\tau = 0.01$, since the method no longer suffers from $\nabla\widetilde{f}_{\boldsymbol{\sigma}}$

going to zero near the boundary. This hypothesis is validated in Figure 2, which shows the data profiles for the subset of 18 CUTEst problems in Appendix C that have at least one constraint active at the solution. In order to solve problems from this subset, PPM must encounter nonsmoothness. Indeed we find that all solvers suffer from handling the bound constraints.

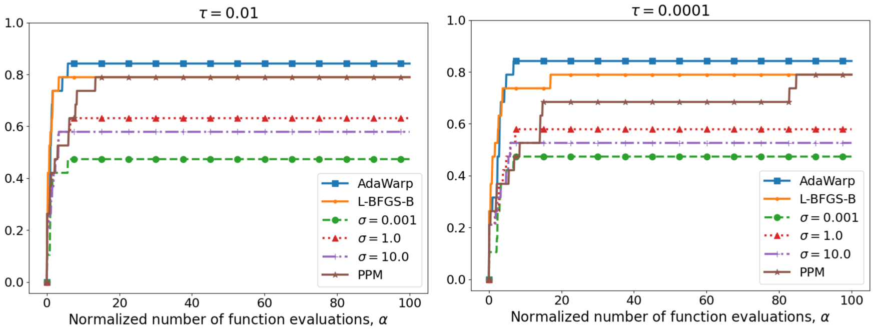


Figure 2: Data profile for a relative KKT tolerance of $\tau = 10^{-2}$ (left) and $\tau = 10^{-4}$ (right) for L-BFGS-B, Algorithm 1 under UPRULE and $\boldsymbol{\sigma}_0 = 10^{-3}$ and L-BFGS as a subproblem solver(labeled AdaWarp), BFGS optimizing $\widetilde{f}_{\boldsymbol{\sigma}}$ with a fixed $\boldsymbol{\sigma}$ (labeled $\boldsymbol{\sigma} = 0.001, 1.0, 10.0$), and the projection-based penalty formulation from [2] solved by [1](labeled PPM). These data profiles are for the set of 18 CUTEst problems with solutions on the boundary of $\boldsymbol{\Omega}$.

# References


[1] N Keskar and A. Wächter. "A limited-memory quasi-Newton algorithm for bound-constrained non-smooth optimization". *Optimization Methods and Software* 34.1 (2019), pp. 150–171. DOI: 10.1080/10556788.2017.1378652.

[2] G. Galvan, M. Sciandrone, and S. Lucidi. "A parameter-free unconstrained reformulation for nonsmooth problems with convex constraints". *Computational Optimization and Applications* 80.1 (2021), pp. 33–53. DOI: 10.1007/s10589-021-00296-1.



The submitted manuscript has been created by UChicago Argonne, LLC, Operator of Argonne National Laboratory ("Argonne"). Argonne, a U.S. Department of Energy Office of Science laboratory, is operated under Contract No. DE-AC02-06CH11357. The U.S. Government retains for itself, and others acting on its behalf, a paid-up nonexclusive, irrevocable worldwide license in said article to reproduce, prepare derivative works, distribute copies to the public, and perform publicly and display publicly, by or on behalf of the Government. The Department of Energy will provide public access to these results of federally sponsored research in accordance with the DOE Public Access Plan http://energy.gov/downloads/doe-public-access-plan.
